# Supplementary material for: GAFusion: Adaptive Fusing LiDAR and Camera with Multiple Guidance for 3D Object Detection
Source: arXiv:2411.00340 source file (2024-11-01)
Supplement: Supplementary file 1 [file X_suppl.tex]

\clearpage
\setcounter{page}{1}
\maketitlesupplementary

\section{Rationale}
\label{sec:rationale}
The supplementary document is organized as follows:
\begin{itemize}
\item The proposed model achieves the results on the Waymo dataset.
% \item More ablation study results; 
\item The generalization study of the proposed LGAFT.
\item Visualization of the model's prediction results in the night-time;
% \item When submitted to arXiv, the supplementary will already included at the end of the paper.
\end{itemize}

%-------------------------------------------------------------------------
\subsection{the results on the Waymo dataset.}
\begin{table}
  \centering
  \begin{adjustbox}{width=0.47\textwidth}
  \begin{tabular}{l|c|cccc}
    \hline
         Methods & Modality & AP/L1 & APH/L1 & AP/L2 & APH/L2 \\
    \hline
    PV-RCNN++ & L & 80.26 & 78.71 & 75.00 & 73.52\\
    MPPNet & L & 81.83 & 80.59 & 76.88 & 75.67\\
    CenterFormer & L & 82.26 & 80.91 & 77.60 & 76.29 \\
   
    \hline
    DeepFusion & LC & 81.90 & 80.48  & 76.91 & 75.54\\
    BEVFusion & LC & 82.72 & 81.35 & 77.65 & 76.33 \\
    % LoGoNet~\cite{yan2023cmt} & LC & 83.14 & 81.83  & 78.38 & 77.10\\
    GAFusion(ours) & LC & \textbf{83.10} & \textbf{81.73}  & \textbf{77.97} & \textbf{76.69}\\
   
    \hline
  \end{tabular}
  \end{adjustbox}
  \caption{Comparison on the Waymo test set. The models in the table are without ensemble or test-time augmentation. }\vspace{-0.2cm}
  \label{tab:waymo_test}
\end{table}
\begin{table}
  \centering
  \begin{adjustbox}{width=0.3\textwidth}
  \begin{tabular}{@{}lccccc@{}}
    \toprule
    & {Class} & {3D obeject} & {2D object}   \\
\midrule
& Vehicle & 6.1M  & 9.0M \\
& Pedestrian & 2.8M  & 2.7M  \\
& Cyclist & 67k  & 81k \\
& Sign & 3.2M  & - \\
    \bottomrule
  \end{tabular}
  \end{adjustbox}
  \caption{The number of 3D and 2D objects of different categories on the Waymo dataset.}\vspace{-0.2cm}
  \label{tab:wamyo_count}
\end{table}

\begin{figure}[t]
  \centering
  % \fbox{\rule{0pt}{2in} \rule{0.9\linewidth}{0pt}}
   %\includegraphics[width=0.8\linewidth]{egfigure.eps}
    \includegraphics[width=\linewidth]{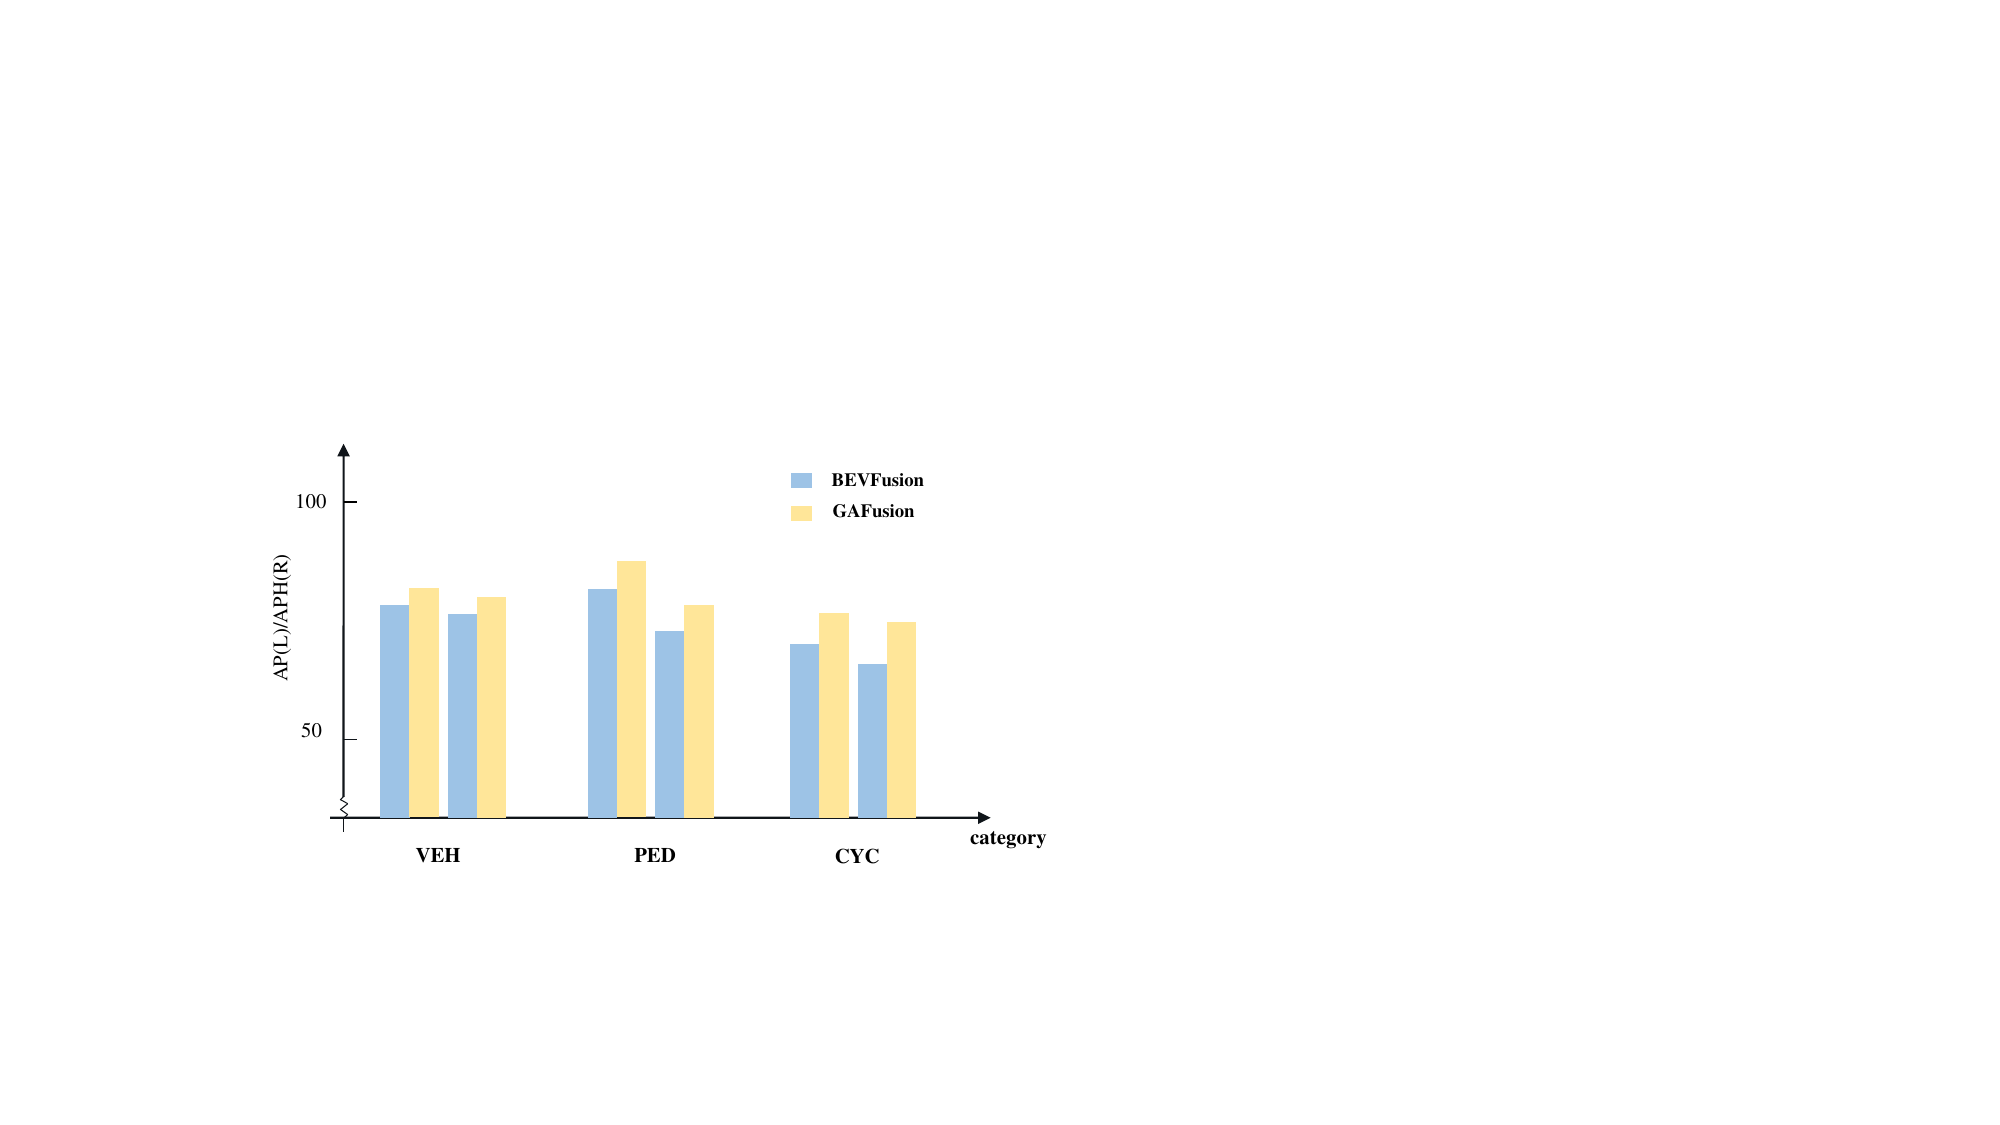}
   \caption{Comparison of BEVFusion and GAFusion on AP/APH (L2)
for each category. For each category, the left is mAP and the right is mAPH. "VEH" is vehicle, "PED" is pedestrian, and "CYC" is cyclist.}
   \label{fig:l2}
\end{figure}

The dataset contains 3,000 driving segments, each of which consists of 20 seconds of continuous driving footage. Each segment covers data from five high-resolution Waymo LiDARs and five front and side cameras. The entire dataset contains a total of 600,000 frames, with about 25 million 3D bounding boxes and 22 million 2D bounding boxes.

As shown in Table~\ref{tab:waymo_test}, we present the results of GAFusion on the Waymo test set and compare it with several models on the Waymo 3D detection leaderboard. We do not use test-time augmentation (TTA) or multi-model ensemble. GAFusion achieves excellent results on the Waymo 3D detection challenge with 76.69 mAPH (L2) detection performance.

In Table~\ref{tab:wamyo_count}, we counted the number of 2D and 3D objects of different categories on the Waymo dataset. It can be seen that there are a large number of relatively small objects (pedestrian, cyclist and sign) on the dataset, which indicates that focusing on the detection accuracy of small objects can benefit the overall performance of the model.

Meanwhile, we compare BEVFusion and the proposed model on vehicle (VEH), pedestrian (PED), and cyclist(CYC) categories in Fig.~\ref{fig:l2}. We observe that GAFusion has a significant improvement over BEVFusion, especially in small and distant objects detection.

%-------------------------------------------------------------------------
\subsection{Generalization of LGAFT module}
\begin{table}
  \centering
  \begin{adjustbox}{width=0.32\textwidth}
  \begin{tabular}{lccll}
    \toprule
    & {Methods} & {LGAFT} & {mAP$\uparrow$} & {NDS$\uparrow$}   \\
\midrule
& BEVFusion & & 70.2  & 72.9 \\
& BEVFusion & \checkmark & 71.0\textcolor[rgb]{0,0.5,0}{$_{\uparrow 0.8}$}  & 73.4\textcolor[rgb]{0,0.5,0}{$_{\uparrow 0.5}$}  \\
\hdashline
& MSMDFusion & & 71.5  & 74.0 \\
& MSMDFusion & \checkmark & 72.1\textcolor[rgb]{0,0.5,0}{$_{\uparrow 0.6}$}  & 74.3\textcolor[rgb]{0,0.5,0}{$_{\uparrow 0.3}$} \\
    \bottomrule
  \end{tabular}
  \end{adjustbox}
  \caption{Generalization of LGAFT module on the nuScenes dataset.}\vspace{-0.2cm}
  \label{tab:study_LGAFT}
\end{table}
To demonstrate the effectiveness and generalization of the proposed module LGAFT, we introduce this module into BEVFusion~\cite{liu2022bevfusion} and MSMDFusion~\cite{jiao2022msmdfusion}. As shown in Table~\ref{tab:study_LGAFT}, with the LGAFT module, BEVFusion achieves a sufficient improvement of 0.8$\%$ mAP and 0.5$\%$ NDS and MSMDFusion brings about 0.6$\%$ mAP and 0.3$\%$ NDS gain. It can be seen that the LGAFT module achieves a relatively significant improvement in different frameworks. This is attributed to the fact that LGAFT can adaptively fuse the BEV features of different modalities from a global perspective, which greatly enhances the interaction of semantic and geometric information and improves the intrinsic correlation between LiDAR and camera.
%-------------------------------------------------------------------------
\subsection{Visualization}

\begin{figure*}[t]
\centering
\includegraphics[width=\textwidth]{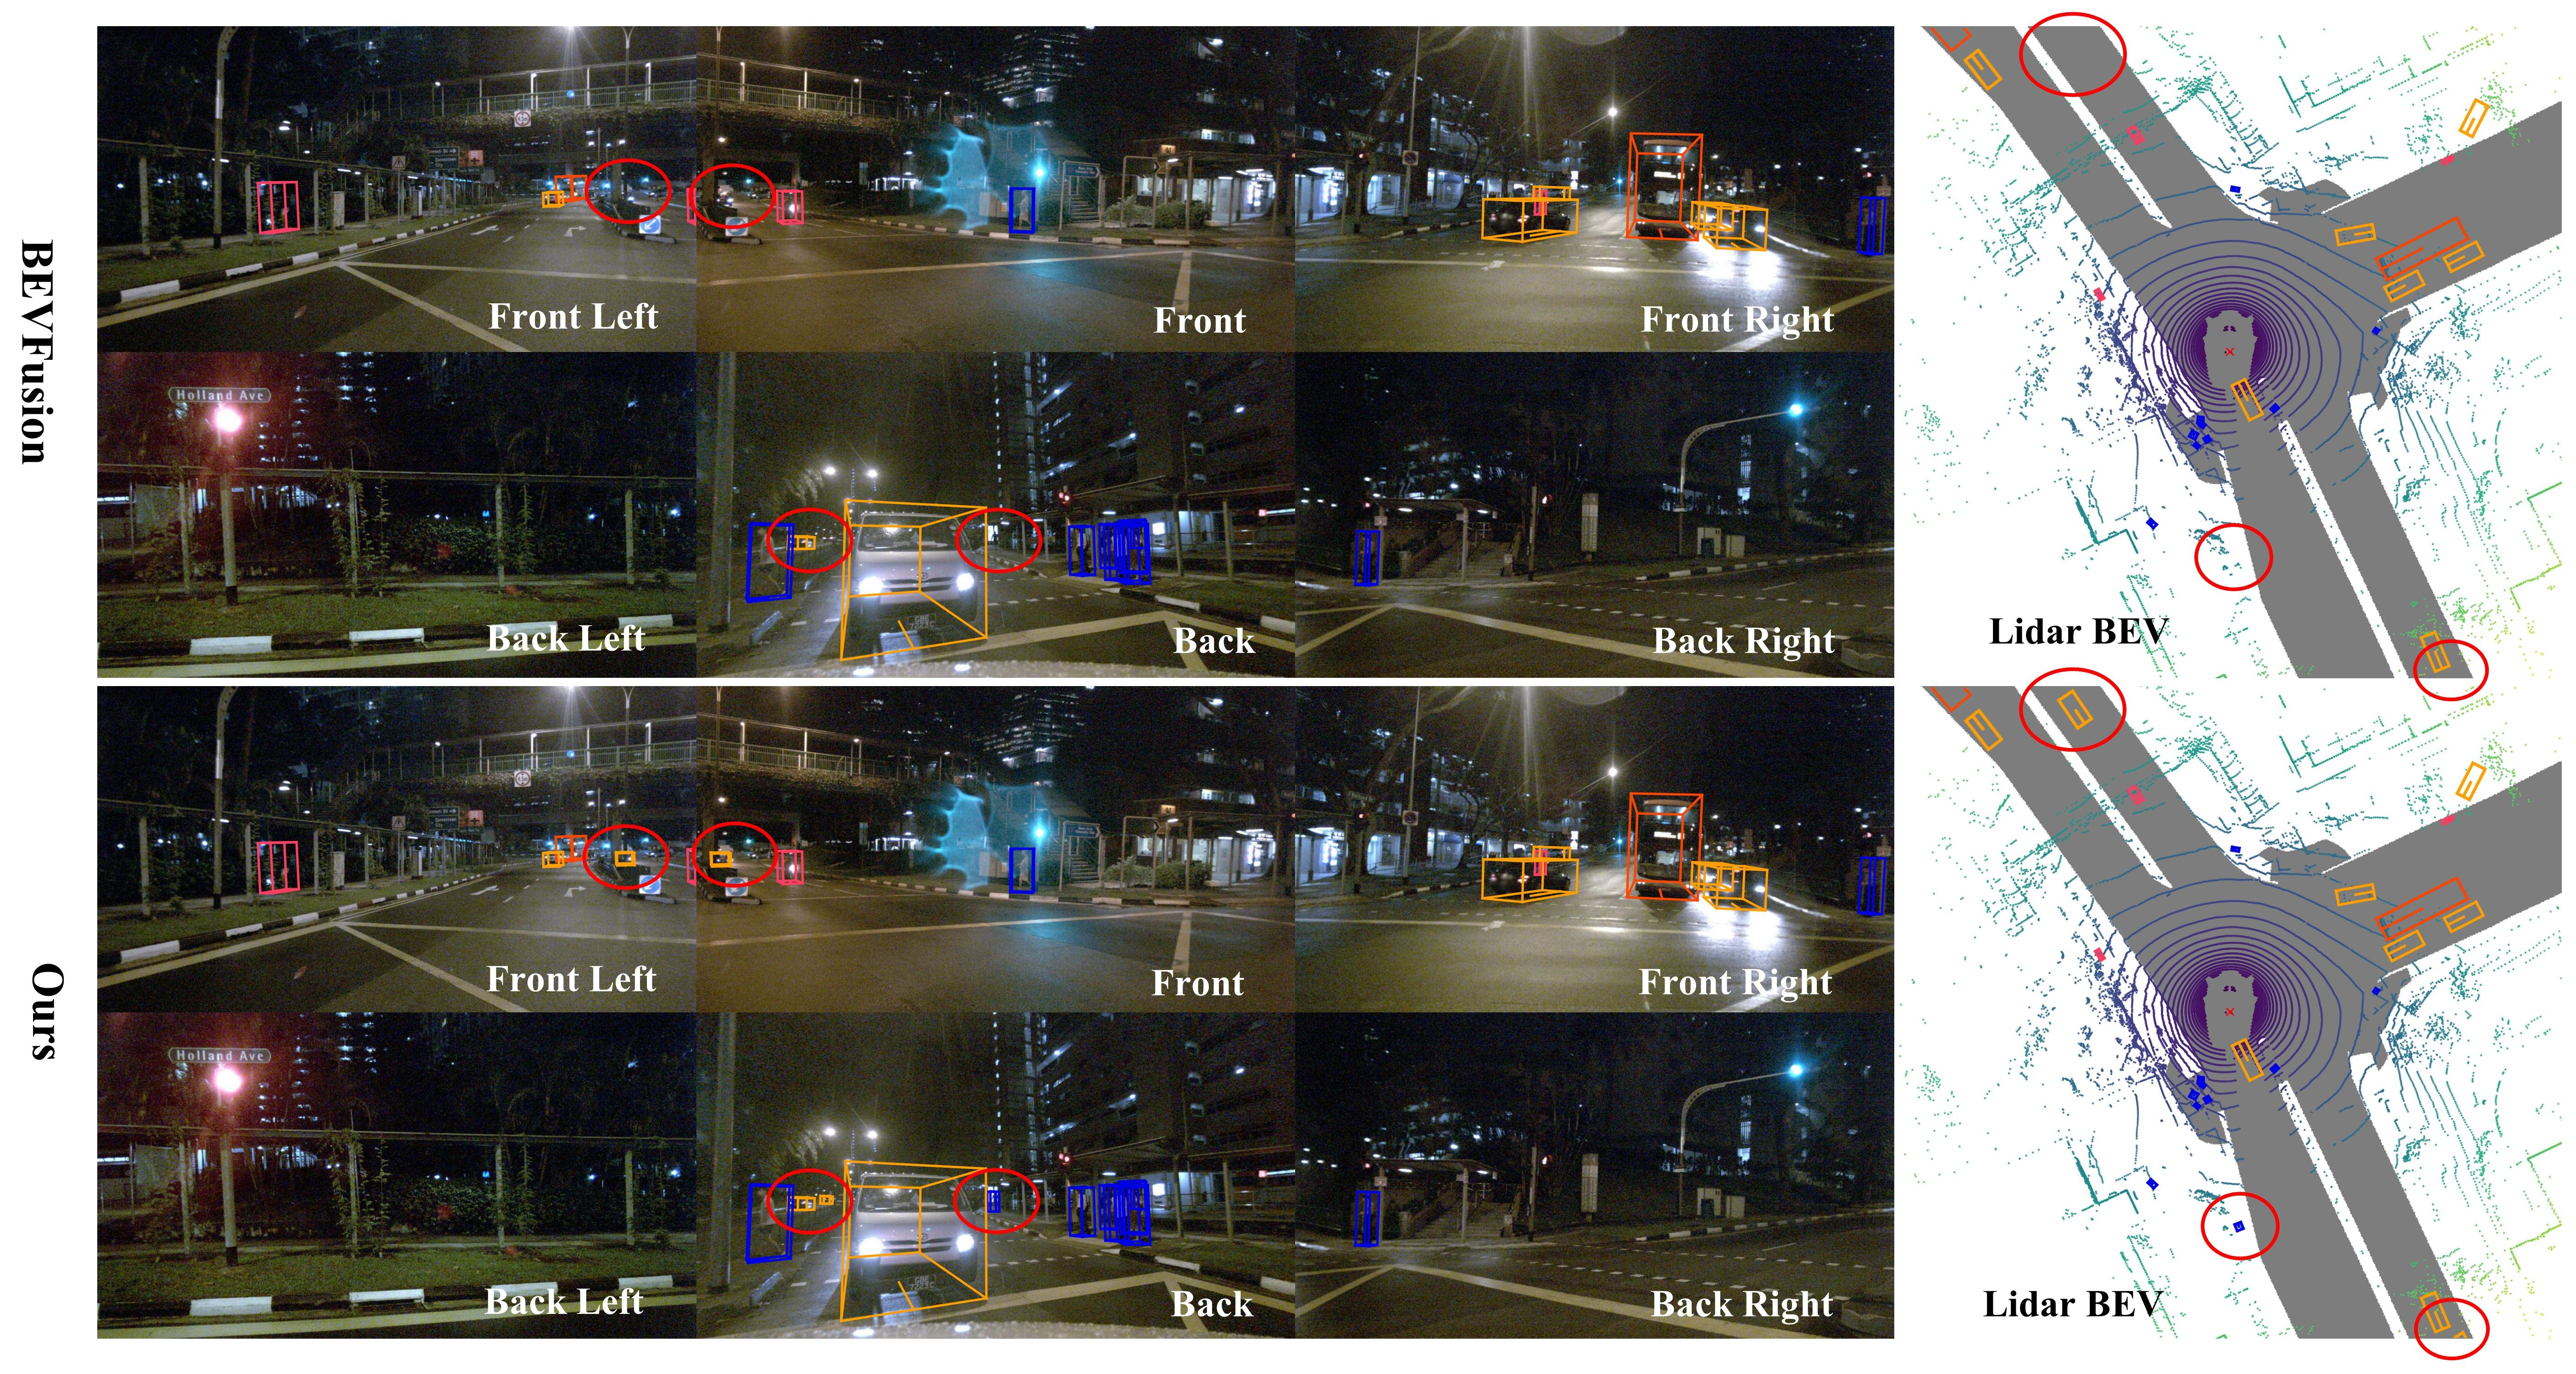}
\caption{Visualization results of BEVFusion and GAFusion at night on the nuScenes validation set. The red circles and boxes show the detection ability of GAFusion for small and occluded objects. }
\label{fig.visual_night} 
\end{figure*}

We show the visualization results on the nuScenes validation set of GAFusion and BEVFusion~\cite{liu2022bevfusion} at night in Fig.~\ref{fig.visual_night}. With the help of our proposed modules, we find that GAFusion achieves excellent performance even at night. This is mainly reflected in its detection performance for distant small objects, which is attributed to better guidance and larger receptive fields.
